# Supplementary material for: Approaching optimality for solving SDD systems
Source: arXiv:1003.2958 source file (2010-08-03)
Supplement: Supplementary file 1 [file appendix.tex]

\section{Sampling} \label{sec:appendix}

The proof uses Theorem~\ref{thm:RudelsonVershynin} below, which is theorem 3.1 from
Rudelson \& Vershynin \cite{RudelsonVershynin07}, the first part of the theorem was
also used as Lemma 5 in \cite{SpielmanSrivastava08} in a similar way:

\begin{theorem}\label{thm:RudelsonVershynin}
Let $p$ be a probability distribution over $\Omega \subseteq R^d$ such that $\sup_{y \in \Omega}||y||_2 \leq M$ and
$ || E_p(yy^T) ||_2 \leq 1$. Let $y_1 \dots y_q$ be independent samples drawn from $p$, and let

$$a := CM\sqrt{\frac{\log{q}}{q}}$$

Then:

\begin{enumerate}

\item $$E||\frac{1}{q} \sum_{i=1}^q y_iy_i^T - E(yy^T)||_2 \leq a$$

\item $$Pr \{ ||\frac{1}{q} \sum_{i=1}^q y_iy_i^T - E(yy^T)||_2 > x \} \leq \frac{2} {e^{cx^2/a^2}}$$

\end{enumerate}

Here $C$ and $c$ are fixed constants.

\end{theorem}

Now consider the matrix:

$$
   \Pi = W^{1/2} B L^{+} B^T W^{1/2}.
$$

We prove the following theorems regarding it:

\begin{theorem}

$\Pi$ is a projection matrix.

\end{theorem}

\Proof

\begin{align*}
\Pi^2 &= W^{1/2} B L^{+} B^T W^{1/2} W^{1/2} B L^{+} B^T W^{1/2}\\
&= W^{1/2} B L^{+} L L^{+} B^T W^{1/2}\\
&= W^{1/2} B L^{+} B^T W^{1/2}\\
&= \Pi
\end{align*}

\QED

\begin{theorem}

Let $S$ by a diagonal matrix. If we multiply the weight of each edge
in $L$ by $S(e,e)$ to get $\tilde{L}$, then
$(1-||\Pi\Pi - \Pi S \Pi||_2)L \preceq \tilde{L} \preceq (1+||\Pi\Pi - \Pi S \Pi||_2)L$.

\end{theorem}

\Proof

We have $L = B^TW^{1/2}W^{1/2}B$ and $\tilde{L} = B^TW^{1/2}SW^{1/2}B$.
Let $x \in \R^n$ such that $x^T1 = 0$, consider $y = W^{1/2}Bx$. Then

\begin{align*}
\Pi y &= W^{1/2} B L^{+} B^T W^{1/2} W^{1/2}Bx \\
&= W^{1/2} B^T L^+ Lx\\
&= W^{1/2} B^T x\\
&= y
\end{align*}

From which we get:

\begin{align*}
& \frac{|x^T\tilde{L}x - x^TLx|}{x^TLx}\\
&= \frac{|y^T B^TW^{1/2}SW^{1/2}B y - y^Ty|}{y^Ty}\\
&= \frac{|y^T\Pi S \Pi y - y^T \Pi\Pi y|}{y^Ty}
\end{align*}

The result then follows by taking max over both sides.

\QED

The conditions of \ref{thm:RudelsonVershynin} can be satisfied as follows: by
setting the probabilities and scaling to ensure edges are scaled by $1/p_e$ when chosen
(which is equivalent to scaling $\Pi(:, e)$ by $\sqrt{1/p_e}$),
we ensure $E(yy^T) = \Pi$, and $||\Pi||_2 \leq 1$ as its a projection matrix. The fact
$\Pi$ is a projection matrix also gives $\Pi(:, e)^T\Pi(:, e) = (\Pi\Pi)(e,e) = \Pi(e,e)$,
which we use to bound $M$:

\begin{align*}
M &= \sup_{e} \frac{1}{\sqrt{p_e}} ||\Pi(:, e)||_2\\
&= \sup_{e} \frac{1}{\sqrt{p_e}} \sqrt{\Pi(e, e)}\\
&= \sup_{e} \frac{1}{\sqrt{p_e}} \sqrt{w_eR_e}` \\
\end{align*}

From which the calculations in ~\ref{thm:sample} follow.
